# Supplementary material for: Model-based clustering for populations of networks
Source: arXiv:1806.00225 source file (2020-01-20)
Supplement: Supplementary file 1 [file supplementary_material.pdf]

Supplementary material for the article
"Model-based clustering for populations of networks"

Mirko Signorelli[1] and Ernst C. Wit[2,3]

[1] *Department of Biomedical Data Sciences, Leiden University Medical Center, The Netherlands*
[2] *Institute of Computational Science, University of Lugano, Switzerland*
[3] *Bernoulli Institute for Mathematics, Computer Science and Artificial Intelligence, University of Groningen, The Netherlands*

# 1 Generation of simulated populations of networks

In simulations A, B and C populations of networks are generated from a mixture of $p_1$ models where

$$y_{ij}^{k}|z_k \sim \text{Bern}\left(\pi_{ij}^{z_k}\right),$$

$$\text{logit}\left(\pi_{ij}^{z_k}\right) = \theta^{z_k} + \alpha_i^{z_k} + \alpha_j^{z_k}$$

where $\theta^{z_k} = -1.4 \ \forall k$ and $\alpha_i \sim U(-0.6, 0.6)$ s.t. $\sum_{i=1}^{v} \alpha_i^{z_k} = 0$.
In simulations D, E and F nodes are split into 3 blocks and populations of networks are generated from a mixture of stochastic blockmodels a priori where

$$\text{logit}\left(\pi_{ij}^{z_k}\right) = \theta_{C(i)C(j)}^{z_k},$$

$C(i) \in \{1, 2, 3\} \ \forall i \in \{1, ..., v\}$ and the block-interaction probability matrices are

$$\begin{bmatrix} 0.4 & 0.1 & 0.1 \\ 0.1 & 0.5 & 0.2 \\ 0.1 & 0.2 & 0.3 \end{bmatrix}, \quad \begin{bmatrix} 0.3 & 0.2 & 0.2 \\ 0.2 & 0.3 & 0.1 \\ 0.2 & 0.1 & 0.4 \end{bmatrix}$$

for the two subpopulations considered in simulation D and E, and

$$\begin{bmatrix} 0.4 & 0.1 & 0.1 \\ 0.1 & 0.4 & 0.1 \\ 0.1 & 0.1 & 0.4 \end{bmatrix}, \begin{bmatrix} 0.55 & 0.1 & 0.1 \\ 0.1 & 0.25 & 0.1 \\ 0.1 & 0.1 & 0.4 \end{bmatrix}, \begin{bmatrix} 0.55 & 0.1 & 0.1 \\ 0.1 & 0.4 & 0.1 \\ 0.1 & 0.1 & 0.25 \end{bmatrix}, \begin{bmatrix} 0.4 & 0.1 & 0.1 \\ 0.1 & 0.55 & 0.1 \\ 0.1 & 0.1 & 0.25 \end{bmatrix},$$

$$\begin{bmatrix} 0.25 & 0.1 & 0.1 \\ 0.1 & 0.55 & 0.1 \\ 0.1 & 0.1 & 0.4 \end{bmatrix}, \begin{bmatrix} 0.25 & 0.1 & 0.1 \\ 0.1 & 0.4 & 0.1 \\ 0.1 & 0.1 & 0.55 \end{bmatrix}, \begin{bmatrix} 0.4 & 0.1 & 0.1 \\ 0.1 & 0.25 & 0.1 \\ 0.1 & 0.1 & 0.55 \end{bmatrix}$$

for the seven subpopulations considered in simulation F.
In simulations G, H, I and J data are generated from a mixture of unconstrained network models where $y_{ij}^k | z_k \sim \text{Bern}\left(\pi_{ij}^{z_k}\right)$ where $\pi_{ij}^{z_k} \sim Beta(\alpha = 2, \beta = 4.67)$ $\forall i < j$, $\pi_{ii}^{z_k} = 0$ and $\pi_{ji}^{z_k} = \pi_{ij}^{z_k}$.
In simulations K and L, populations of networks are generated from a mixture of stochastic blockmodels a priori where

$$\text{logit}\left(\pi_{ij}^{z_k}\right) = \theta_{C(i)C(j)}^{z_k},$$

$C(i) \in \{1, 2, 3, 4, 5\}$ $\forall i \in \{1, ..., v\}$, and the block-interaction probabilities are randomly drawn from a uniform distribution ranging in $[0.2, 0.5]$ for diagonal elements ($\theta_{rr}^{z_k}$) and in $[0.02, 0.15]$ for off-diagonal elements ($\theta_{rs}^{z_k}$, $r \neq s$).

# 2 Supplementary figures

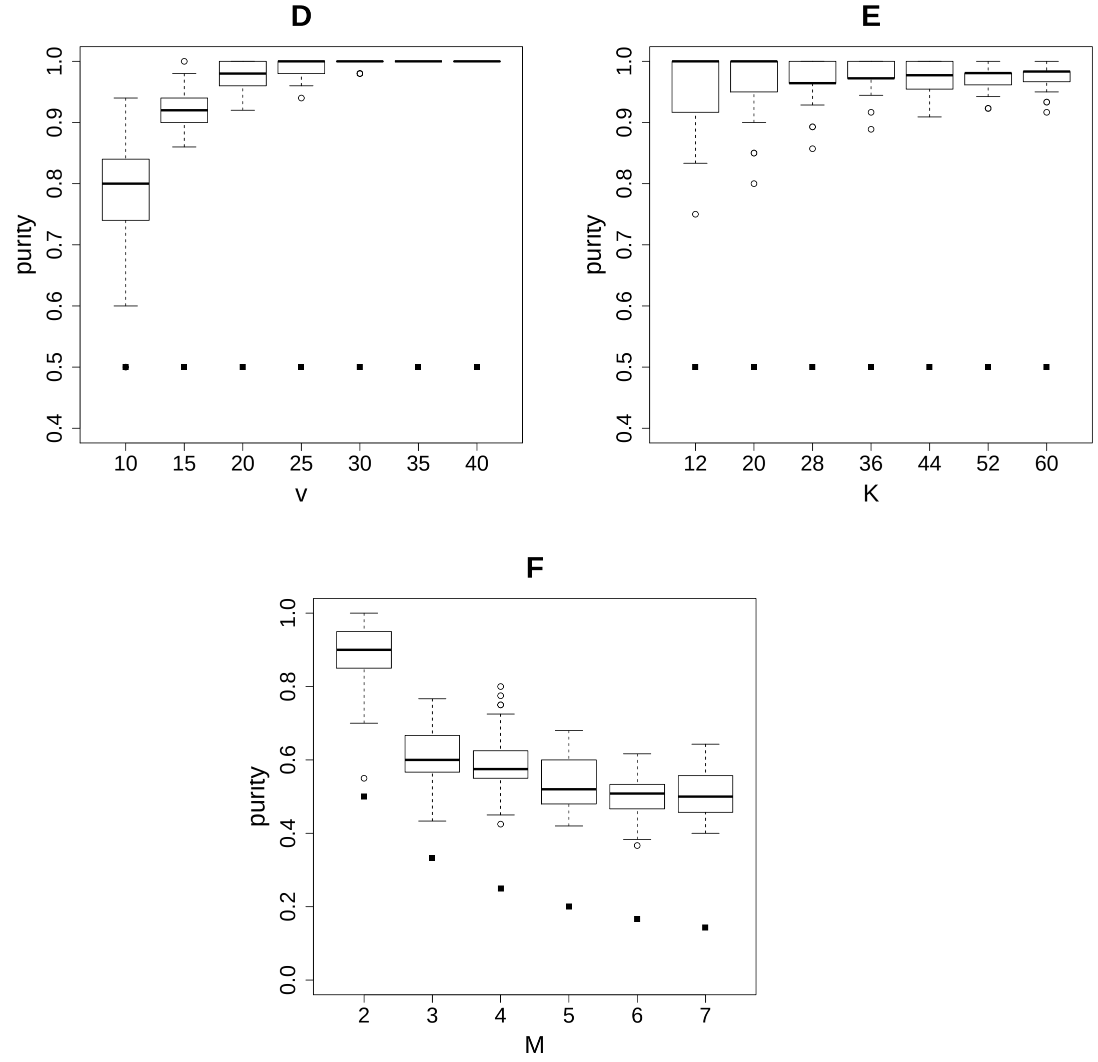


Figure 1: Purity in simulations D, E, F. Each boxplot represents the distribution of purity over 50 repetitions, whereas the squares denote the value of purity that corresponds to a random assignment of graphs to clusters (i.e., $1/M$).

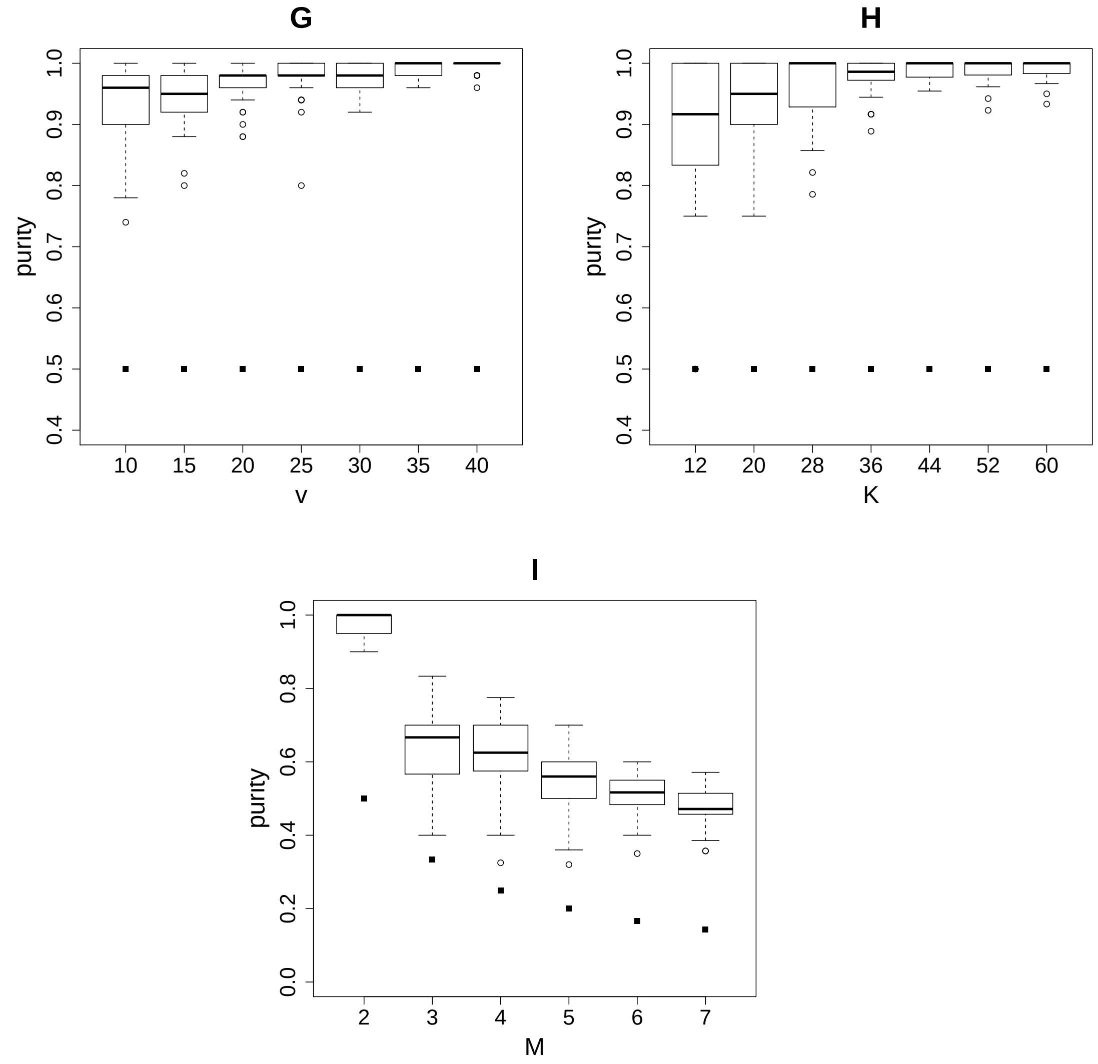


Figure 2: Purity in simulations G, H, I. Each boxplot represents the distribution of purity over 50 repetitions, whereas the squares denote the value of purity that corresponds to a random assignment of graphs to clusters (i.e., $1/M$).

# 3 Parameter estimates for the departments' main effect and interaction parameters

Table 1: Maximum likelihood estimates and standard errors for the covariates in model (5.1). * indicates parameters that are significantly different from 0 at $\alpha = 5\%$ level. The last column contains the p-value of the test for equality of each parameter in the two subpopulations.

| Parameter | $\hat{\theta}^1$ | $\hat{\theta}^2$ | $SE(\hat{\theta}^1)$ | $SE(\hat{\theta}^2)$ | p-value ($\theta^1 = \theta^2$) |
|---|---|---|---|---|---|
| $\gamma_1$ | -0.217 | -0.346* | 0.167 | 0.132 | 0.593 |
| $\gamma_2$ | 0.167 | 0.350* | 0.177 | 0.140 | 0.453 |
| $\gamma_3$ | 0.246 | -0.043 | 0.201 | 0.156 | 0.248 |
| $\gamma_4$ | -0.196 | 0.039 | 0.167 | 0.132 | 0.329 |
| $\delta_1$ | -0.109 | -0.324* | 0.216 | 0.121 | 0.391 |
| $\delta_2$ | -0.329 | -0.194 | 0.234 | 0.133 | 0.600 |
| $\delta_3$ | 0.335 | 0.210 | 0.264 | 0.140 | 0.637 |
| $\delta_4$ | 0.102 | 0.308* | 0.177 | 0.140 | 0.397 |
| $\xi_{11}$ | 1.972* | 1.732* | 0.179 | 0.118 | 0.321 |
| $\xi_{21}$ | -0.826* | -0.773* | 0.132 | 0.108 | 0.818 |
| $\xi_{31}$ | -1.108* | -0.769* | 0.184 | 0.154 | 0.169 |
| $\xi_{41}$ | -0.038 | -0.189 | 0.161 | 0.127 | 0.526 |
| $\xi_{12}$ | -0.530* | -0.508* | 0.143 | 0.127 | 0.925 |
| $\xi_{22}$ | 1.215* | 1.250* | 0.119 | 0.092 | 0.880 |
| $\xi_{32}$ | 0.421* | 0.080 | 0.162 | 0.130 | 0.155 |
| $\xi_{42}$ | -1.106* | -0.822* | 0.161 | 0.131 | 0.235 |
| $\xi_{13}$ | -1.278* | -1.171* | 0.196 | 0.151 | 0.667 |
| $\xi_{23}$ | 0.300 | 0.128 | 0.167 | 0.109 | 0.473 |
| $\xi_{33}$ | 0.665* | 1.069* | 0.276 | 0.160 | 0.134 |
| $\xi_{43}$ | 0.313 | -0.026 | 0.205 | 0.136 | 0.173 |
| $\xi_{14}$ | -0.164 | -0.053 | 0.165 | 0.125 | 0.643 |
| $\xi_{24}$ | -0.689* | -0.605* | 0.144 | 0.105 | 0.722 |
| $\xi_{34}$ | 0.022 | -0.380 | 0.200 | 0.146 | 0.106 |
| $\xi_{44}$ | 0.830* | 1.038* | 0.194 | 0.129 | 0.400 |
